# Supplementary material for: Scaling Ensemble Distribution Distillation to Many Classes with Proxy Targets
Source: arXiv:2105.06987 source file (2021-05-14)
Supplement: Supplementary file 1 [file appendix.tex]

\section{Derivations} \label{apn:derivations}

The current section details the derivation of differential entropy, mutual information and expected pairwise KL-divergence for a Prior Network which parameterizes the Dirichlet distribution:
\begin{empheq}{align}
\begin{split}
{\tt p}(\bm{\pi} | \bm{x}^{*};\bm{\hat \theta}) =&\ {\tt Dir}(\bm{\pi} ; \bm{\hat \alpha}) \\
\bm{\hat \alpha} =&\ \bm{f}(\bm{x}^{*};\bm{\hat \theta})
\end{split}
\end{empheq}
where ${\tt p}(\bm{\pi} ; \bm{\hat \alpha})$ is a prior distribution over categorical distributions.
The Dirichlet distribution is defined as:
\begin{empheq}{align}
\begin{split}
{\tt Dir}(\bm{\pi};\bm{\alpha}) =&\ \mathcal{C}(\bm{\alpha})\prod_{c=1}^K \pi_c^{\alpha_c -1} ,\quad \alpha_c >0\\
\mathcal{C}(\bm{\alpha}) =&\  \frac{\Gamma(\alpha_0)}{\prod_{c=1}^K\Gamma(\alpha_c)},\quad \alpha_0 = \sum_{c=1}^K \alpha_c
\end{split}
\end{empheq}
where $\Gamma(\cdot)$ is the \emph{Gamma function}.

\subsection{Differential Entropy}
The differential entropy of the Dirichlet distribution can be derived as follows:
\begin{empheq}{align}
\begin{split}
  \mathcal{H}[{\tt p}(\bm{\pi}|\bm{x}^{*};\bm{\hat \theta})]=&\ -\mathbb{E}_{{\tt p}(\bm{\pi}|\bm{x};\bm{\hat \theta})}[\ln({\tt p}(\bm{\pi}|\bm{x};\bm{\hat \theta}))] \\
=&\ \sum_{c=1}^K\ln\Gamma(\hat \alpha_c)-\ln\Gamma(\hat \alpha_0) - \sum_{c=1}^K(\hat \alpha_c-1)\mathbb{E}_{{\tt p}(\bm{\pi}|\bm{x};\bm{\hat \theta})}[\ln\pi_c] \\
=&\ \sum_{c=1}^K\ln\Gamma(\hat \alpha_c)-\ln\Gamma(\hat \alpha_0) - \sum_{c=1}^K(\hat \alpha_c-1)\cdot\big(\psi(\hat \alpha_c)-\psi(\hat \alpha_0)\big)
\end{split}
\end{empheq}
where $\psi$ is the \emph{digamma function} and $\mathbb{E}_{{\tt p}(\bm{\pi}|\bm{\hat \alpha})}[\ln(\pi_c)]=\psi(\hat \alpha_c)-\psi(\hat \alpha_0)$ is a standard result.

\subsection{Mutual Information}
The mutual information between the labels y and the categorical $\bm{\pi}$ for a Dirichlet distribution can be calculated as follows, using the fact that mutual information is the difference of the entropy of the expected distribution and the expected entropy of the distribution.
\begin{empheq}{align}
\begin{split}
\underbrace{\mathcal{I}[y,\bm{\pi} |\bm{x}^{*},\bm{\hat \theta}]}_{Knowledge\ Uncertainty} = &\  \underbrace{\mathcal{H}[ \mathbb{E}_{{\tt p}(\bm{\pi}|\bm{x}^{*}, \bm{\hat \theta})}[{\tt P}(y|\bm{\pi}]]}_{Total\ Uncertainty} - \underbrace{\mathbb{E}_{{\tt p}(\bm{\pi}|\bm{x}^{*}, \bm{\hat \theta})}[\mathcal{H}[{\tt P}(y|\bm{\pi})]]}_{Expected\ Data\ Uncertainty} \\
= &\ \mathcal{H}[{\tt P}(y|\bm{x}^{*},\bm{\hat \theta})]  + \sum_{c=1}^K \mathbb{E}_{{\tt p}(\bm{\pi}|\bm{x}^{*}, \bm{\hat \theta})}[\pi_c\ln\pi_c] \\
=&\ -\sum_{c=1}^K\frac{\hat \alpha_c}{\hat \alpha_0}\Big(\ln\frac{\hat \alpha_c}{\hat \alpha_0} - \psi(\hat \alpha_c+1) +\psi(\hat \alpha_0+1) \Big)
\end{split}
\end{empheq}
The second term in this derivation is a non-standard result. The expected entropy of the distribution can be calculated in the following way:
\begin{empheq}{align}
\begin{split}
\mathbb{E}_{{\tt p}(\bm{\pi}|\bm{x}^{*}, \bm{\hat \theta})}[\pi_c\ln\pi_c] = &\ \frac{\Gamma(\hat \alpha_0)}{\prod_{c=1}^K\Gamma(\hat \alpha_c)}\int_{\mathcal{S}_K}\pi_c\ln\pi_c\prod_{c=1}^K \pi_c^{\hat \alpha_c -1}d\bm{\pi}   \\
= &\ \frac{\hat \alpha_c}{\hat \alpha_0}\frac{\Gamma(\hat \alpha_0+1)}{\Gamma(\hat \alpha_c+1)\prod_{c'=1, \neq c}^K\Gamma(\hat \alpha_{c'})}\int_{\mathcal{S}_K}\pi_c^{\hat \alpha_c}\ln\pi_c\prod_{c'=1,\neq c}^K \pi_{c'}^{\hat \alpha_{c'} -1}d\bm{\pi} \\
= &\ \frac{\hat \alpha_c}{\hat \alpha_0}\big(\psi(\hat \alpha_c+1) - \psi(\hat \alpha_0+1)\big)
\end{split}
\end{empheq}
Here the expectation is calculated by noting that the standard result of the expectation of $\ln\pi_c$ with respect to a Dirichlet distribution can be used if the extra factor $\pi_c$ is accounted for by adding 1 to the associated concentration parameter $\hat \alpha_c$ and multiplying by $\frac{\hat \alpha_c}{\hat \alpha_0}$ in order to  have the correct normalizing constant.

\subsection{Expected Pairwise KL-divergence}
Similarly, the Expected Pairwise KL-divergence can also be analytically calculated for the Dirichlet distribution using the following derivation:
\begin{empheq}{align}
\begin{split}
\mathcal{K}[{\tt p}(\bm{\pi}|\bm{x}^{*};\bm{\hat \theta})] = &\ \mathbb{E}_{{\tt p}(\bm{\pi}^{(1)}|\bm{x}^{*};\bm{\hat \theta}),{\tt p}(\bm{\pi}^{(2)}|\bm{x}^{*};\bm{\hat \theta})}\big[{\tt KL}[{\tt P}(y|\bm{\pi}^{(1)})||{\tt P}(y|\bm{\pi}^{(2)})]\big] \\
= &\ - \sum_{c=1}^K\mathbb{E}_{{\tt p}(\bm{\pi}^{(1)}|\bm{x}^{*};\bm{\hat \theta})}[{\tt P}(\omega_c|\bm{\pi}^{(1)})]\mathbb{E}_{{\tt p}(\bm{\pi}^{(2)}|\bm{x}^{*};\bm{\hat \theta})}[\ln {\tt P}(\omega_c|\bm{\pi}^{(2)})] \\
- &\ \mathbb{E}_{{\tt p}(\bm{\pi}^{(1)}|\bm{x}^{*};\bm{\hat \theta})}\big[\mathcal{H}[{\tt P}(y|\bm{\pi}^{(1)})]\big] \\
= &\  \sum_{c=1}^K\mathbb{E}_{{\tt p}(\bm{\pi}|\bm{x}^{*};\bm{\hat \theta})}[\pi_c\ln\pi_c] - \sum_{c=1}^K\mathbb{E}_{{\tt p}(\bm{\pi}|\bm{x}^{*};\bm{\hat \theta})}[\pi_c]\mathbb{E}_{{\tt p}(\bm{\pi}|\bm{x}^{*};\bm{\hat \theta})}[\ln\pi_c]
\end{split}
\end{empheq}
The last step is valid only if ${\tt p}(\bm{\pi}^{(1)}|\bm{x}^{*};\bm{\hat \theta}) = {\tt p}(\bm{\pi}^{(2)}|\bm{x}^{*};\bm{\hat \theta}) = {\tt p}(\bm{\pi}|\bm{x}^{*};\bm{\hat \theta})$, which represents independent draws of categorical from the Dirichlet. This expression then leads to a particularly elegant solution:
\begin{empheq}{align}
\begin{split}
\mathcal{K}[{\tt p}(\bm{\pi}|\bm{x}^{*};\bm{\hat \theta})] = &\  \sum_{c=1}^K\frac{\hat \alpha_c}{\hat \alpha_0}\big(\psi(\hat \alpha_c+1) -\psi(\hat \alpha_0+1)\big) - \sum_{c=1}^K\frac{\hat \alpha_c}{\hat \alpha_0}\big(\psi(\hat \alpha_c)-\psi(\hat \alpha_0)\big) \\
= &\  \frac{K-1}{\hat \alpha_0}
\end{split}
\end{empheq}
Thus, the expected pairwise KL-divergence is inversely proportional to the concentration of the Dirichlet and is maximized when the concentration $\hat \alpha_0$ tends to 0.
